# Supplementary material for: A Surprisingly Robust Trick for Winograd Schema Challenge
Source: arXiv:1905.06290 source file (2019-08-04)
Supplement: Supplementary file 1 [file appendix.tex]

\section*{Appendix}
\subsection*{Dataset Filtering Procedure}
We filter the dataset to reduce the number of ``simple'' examples, while capturing the ``harder'' ones.
Let $\mathbf{s}$ denote a masked sentence, and let $c_1, c_2$ be the correct and incorrect candidate, respectively.
For each example, $\log\mathbb{P}(c_1|\mathbf{s})$ and $\log\mathbb{P}(c_2|\mathbf{s})$ are computed using \textsc{Bert\_WscR}. 
We observe the value $v=\log\mathbb{P}(c_2|\mathbf{s})-\log\mathbb{P}(c_1|\mathbf{s})$.

We manually observe $1000$ randomly selected examples to determine how $v$ relates to the quality of the example.
More specifically, examples where one option is grammatically incorrect or is visibly a better choice than the other, are considered ``easy'', and the examples where reasoning or understanding is needed to solve them are considered ``hard''.
A more detailed description of this criterion is included below.

We pick the examples with $-0.075\leq v \leq 0.30$, where at least $90\%$ of WordPiece tokens \cite{WordPiece} represent whole words.
The upper bound was necessary, because \textsc{Bert\_WscR} scored some incorrect examples as having high $\mathbb{P}(c_2|\mathbf{s})$, just because the correct solution was a really rare word, for example, a non-English surname with non-ASCII characters (hence, its predicted $\mathbb{P}(\mathbf{c}_1|\mathbf{s})$ was low).
The boundary values were selected manually to retain hard examples and filter out the easy ones, based on manual inspection of the mentioned random subset.
After filtering, the final dataset consists of $11,700,317$ out of a total of $129,852,279$ examples, i.e., we kept $9\%$ of the initially generated dataset.

To determine the quality of the dataset, $200$ random examples are manually categorized into $4$ categories:
\begin{itemize}
  \vspace*{-1ex}  \item Unsolvable: the masked word cannot be unambiguously selected with the given context. Example:
    \textit{Mostly shot in Australia and South Africa, the film is based on the controversy regarding the allegedly racial attacks on Indian students in [MASK] between 2007 and 2010. [Australia/South Africa]}
  \vspace*{-1ex}  \item Hard: the answer is not trivial to figure out, but we do not require it to pass the Google test. Example: \textit{The heavy grazing by the cattle resulted stoppage of regeneration of new grasses due to no seeding of seeds and trampling of new [MASK]. [grasses/seeds]}%\textit{After retreating to the safety at the Papaya Plateau , Wang Bingxiang heard gunshots in the direction of Peach Tree Village , and he immediately led his guerrilla to the direction of [MASK] to reinforce their comrades.[gunshots,Papaya Plateau]}
  \vspace*{-1ex}  \item Easy: The alternative sentence is grammatically incorrect or is very visibly an inferior choice. Example: \textit{``Stay on These Roads" achieved Platinum status in Brazil and Gold in the UK, Switzerland, the Netherlands and Germany and Double [MASK] in France. [Platinum Status/Switzerland]}
  \vspace*{-1ex}  \item Noise: The example is a result of a parsing error.% Example: \textit{In batting , he had 49 at - bats in 30 games , [MASK]. [batting,bats]}
\end{itemize}
In the analyzed subset, $12\%$ of examples were unsolvable, $53\%$ were hard, $34\%$ were easy, and $1\%$ fell into the noise category.

\subsection*{Evaluation on \textsc{Wnli}}
Models are additionally tested on the test partition of the \textsc{Wnli} dataset.
To use the same evaluation approach as for the \textsc{Wsc273} dataset, the examples in \textsc{Wnli} have to be transformed from the premise--hypothesis format into the masked words format.
Since each hypothesis is just a sub-string of the premise with the pronoun replaced for the candidate, finding the replaced pronoun and one candidate can be done by finding the hypothesis as a sub-string of the premise.
All other nouns in the sentence are treated as alternative candidates.
The Stanford POS-tagger \cite{StanfordPOS} is used to find the nouns in the sentence.
The probability for each candidate is computed to determine whether the candidate in the hypothesis is the best match.
Only the test partition of the \textsc{Wnli} dataset is used, because it does not overlap with \textsc{Wsc273}.
We do not train or validate on the \textsc{Wnli} training and validation sets, because some of the examples share the premise. Indeed, when upper rephrasing of the examples is used, the training, validation, and test sets start to overlap.
